# Supplementary material for: High Harmonic Generation in Two-Dimensional Mott Insulators
Source: arXiv:2103.13708 ancillary file (2021-07-26)
Supplement: Supplementary file 1 [file supplementary_materials.pdf]

# Supplementary Material for "High Harmonic Generation in Two-Dimensional Mott Insulators"

## HUBBARD LATTICE

The Hilbert space of configurations in half-filled lattices used in this work for Mott regimes scales as  $\left(\frac{L}{L/2}\right)^2$ , where  $L$  is the number of sites (accounting for particle number and spin-polarization symmetry). This limits high harmonic generation (HHG) calculations using ED to 12 sites. The square lattice is the natural 2D extension to the 1D chain, and we would like to simulate this in the thermodynamic limit. However, for a simple  $4 \times 3$  square lattice with periodic boundary conditions, we observe an artificial phase transition in the ground state at  $U \sim 6t_0$ . This is an artifact of the small system size, inducing frustration in the y-direction prohibits the formation of antiferromagnetic order (AFM). We verified via comparison to VMC that this disappears for systems with 16 or more sites, which means that more care was needed for a faithful description of 2D dynamics with these small lattices. We found that the equivalent tilted lattice system, with unit cell (4,0) (3,3), does not develop frustration and can support perfect AFM, and therefore does not undergo a ground state phase transition. For this reason this tilted system is used for the results of Fig. 1, as it is more representative of the square system in the thermodynamic limit, and was benchmarked against VMC in larger lattices.

While the main paper observes the dynamical Mott photo-transition of the ground state order via the density of doublons, this can also be observed by directly probing the spin correlations, defined as

$$\eta = \frac{1}{dL} \sum_{\langle i,j \rangle} \langle \hat{\mathbf{S}}_i \cdot \hat{\mathbf{S}}_j \rangle \quad (1)$$

for dimension  $d$  and total number of lattice sites  $L$ . The interacting ground state at half filling possesses antiferromagnetic order which is destroyed by the pulse, resulting in a paramagnetic state. This is observed in Supplementary Fig. 1, which shows the evolution of  $\eta$  and its dependence on correlation and dimensionality, again with a tilted 2D lattice. It is clear that in 2D the Mott transition occurs more rapidly after irradiation than in 1D, as was observed in the spectrogram of Fig. 3.

## EFFECTIVE SINGLE-PARTICLE MODEL Bandstructure

The spectral function for the effective single-particle model subject to dynamical renormalization of the bandstructure is given by

$$A(\omega) = -\frac{1}{\pi L} \text{Tr} [\text{Im} \{G(\omega + i\epsilon)\}] \quad (2)$$

where  $\epsilon$  is a small, positive broadening parameter. The one-body Green's function is  $G(\omega) = P(\omega\mathbb{1} - \hat{h})^{-1}P$ ,

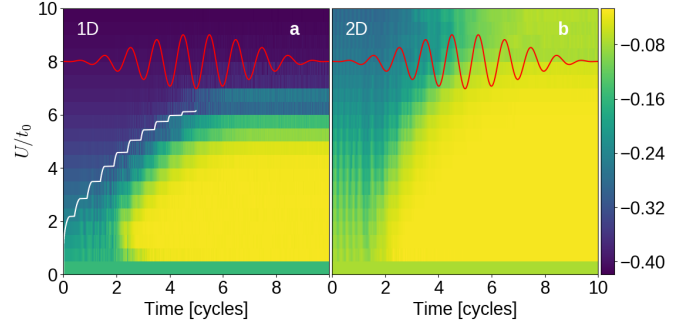

**Supplementary Fig. 1. Demonstration of photo-induced Mott transition.** Plot shows the evolution of the spin-spin correlation function in the 1D (a) and 2D (b) Hubbard models as  $U/t_0$  is varied. Both systems are comprised of 12-site lattices, calculated by ED. The white line shows the time that the threshold field  $E_{th}$  is exceeded, using analytic expressions for the Mott gap and coherence lengths in the thermodynamic limit, available in 1D from the Bethe ansatz.

where  $\hat{h}$  is the Hamiltonian of the physical  $\oplus$  auxiliary system, as defined in the Methods section of the main text, and  $P$  is a projection operator into the physical lattice, allowing the auxiliary system to be traced out. Supplementary Fig. 2 shows the ground-state bandstructure for this effective model after optimization of the  $V(U)$  parameter, for the effective correlation strengths of  $U/t_0 = 0, 3, 7$  in 1D and 2D.  $V > 0$  leads to the formation of a gap separating occupied ( $\omega < \mu$ ) and unoccupied ( $\omega > \mu$ ) states, representing the minimum energy required to create excitations in the ground state system. The set of available excitations is then an important factor in the high harmonic emission following irradiation. The momentum-allowed spectral range of excitations in the 1D Fermi-Hubbard model are given by  $\Delta$  to  $\Delta + 8t_0$ , with the Mott gap,  $\Delta(U)$  known semi-analytically as [1]

$$\Delta = \frac{16t_0^2}{U} \int_1^\infty \frac{\sqrt{y^2 - 1}}{\sinh(2\pi y t_0/U)} dy. \quad (3)$$

In 2D there is no known analytic expression, but in the non-interacting model eq. (2) can be used to approximate the bandstructure and therefore the gap, and to study how it changes with correlation and dimensionality. The model predicts that the Mott gap is smaller in 2D for all interaction strengths, as is visible in Supplementary Fig. 2, and corroborated by cluster perturbation theory results [2, 3].

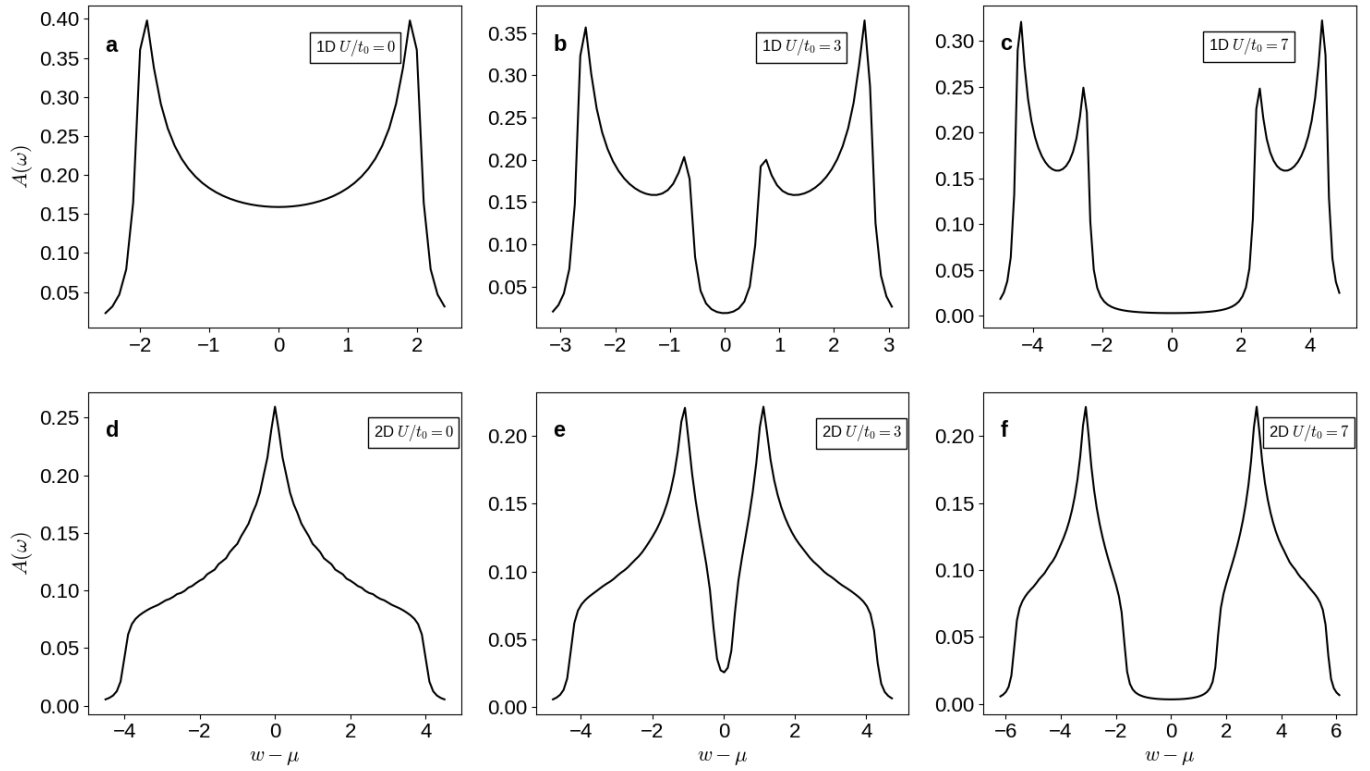

**Supplementary Fig. 2. Effects of correlation and dimensionality on the effective renormalized model band-structure.** Spectral function estimated using the effective correlated model, with  $\epsilon = 0.1t_0$  in 1D (a-c) and 2D (d-f), for  $U/t_0 = 0, 3, 7$ .

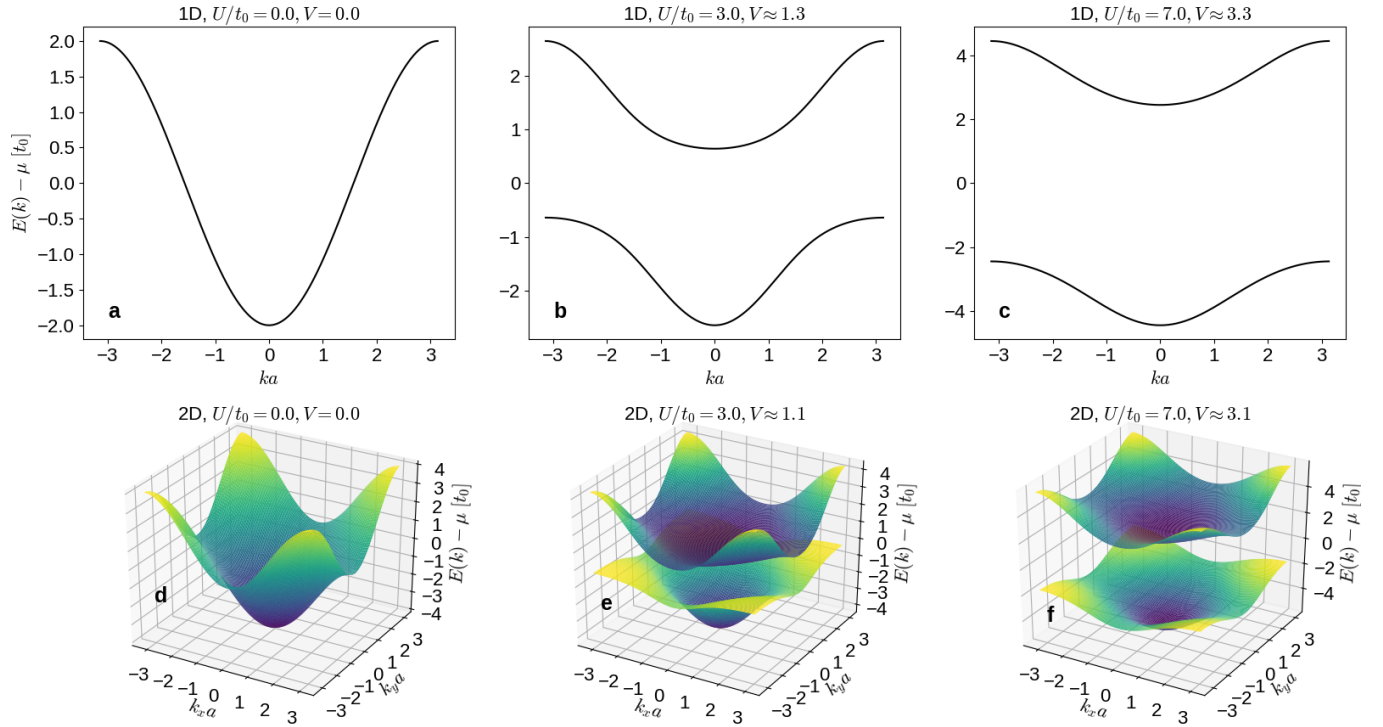

**Supplementary Fig. 3. Band structures in the effective single-particle model.** Energy as a function of quasi-momentum in 1D (a-c) and 2D (d-f). Shown for  $U/t_0 = 0, 3, 7$ , corresponding in 1D to  $V \approx 0, 1.3, 3.3$  and in 2D to  $V \approx 0, 1.1, 3.1$ .

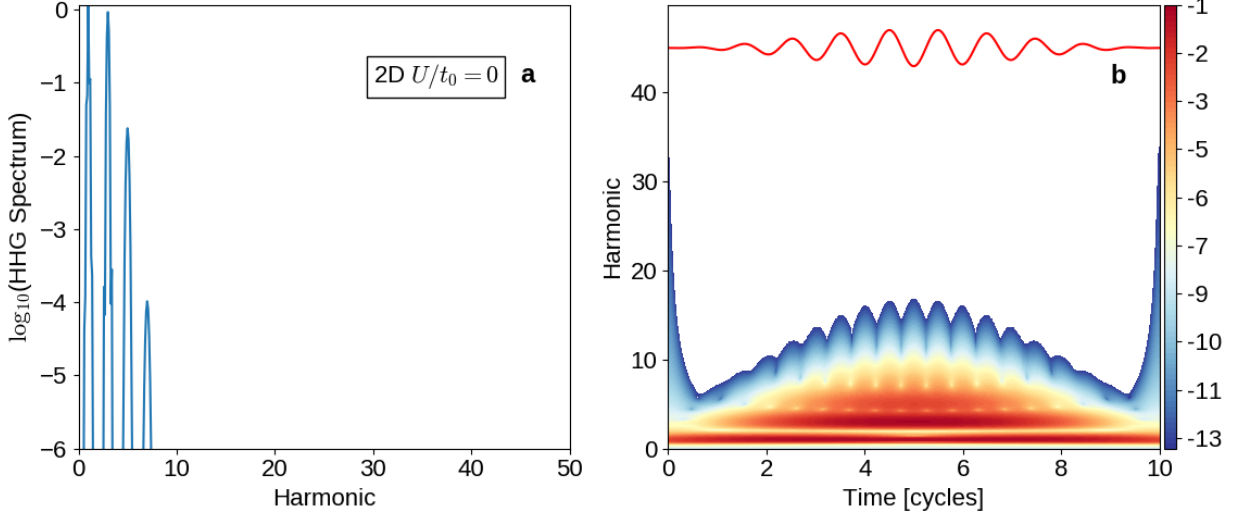

**Supplementary Fig. 4. Time-averaged and time-frequency resolved emission in 2D in the absence of correlation.** HHG for  $U/t_0 = V = 0$ . The red curve shows the electric field,  $E(t) = -dA(t)/dt$

The dispersion can be calculated by Fourier transforming eq. (14). This leads to

$$E(\mathbf{k}) = \frac{1}{2} \left( \alpha(\mathbf{k}) \pm \sqrt{\alpha(\mathbf{k})^2 + 4\beta(\mathbf{k})} \right), \quad (4)$$

where

$$\alpha(\mathbf{k}) = \epsilon(\mathbf{k}) - U \quad (5)$$

$$\beta(\mathbf{k}) = V^2(U) + \left( \epsilon(\mathbf{k}) - \frac{U}{2} \right) \frac{U}{2}, \quad (6)$$

and  $\epsilon(\mathbf{k}) = -2t_0 \sum_{n=1}^d \cos[\mathbf{k}_n a]$  for dimension  $d$  is the dispersion of the  $U = 0$  Hubbard Hamiltonian (the tight-binding model). Supplementary Fig. 3 shows eq. (4) in 1D and 2D.

### High harmonic emission

Supplementary Fig. 4 shows emission in the 2D tight-binding model, where  $U/t_0 = 0$  (i.e.  $V = 0$ ), in the Fermi liquid regime. In this case there is no Mott gap and therefore no recombination of excited states, so the emission originates purely from Bloch oscillations. This produces distinct sharp peaks concentrated below the 10th harmonic, and emission intensity that is aligned in time with the field strength. The HHG changes significantly in the correlated-bandstructure model due to the opening of a Mott gap. An upper Hubbard band allows for emission at much larger harmonics and introduces a complex interplay between intra- and inter-band processes, not least because the availability of excited states determines whether or not the system is actually able to support intra-band currents.

As discussed in the main text, this non-interacting model does not have AFM order in the ground state and

therefore cannot undergo a Mott transition at any  $V(U)$ . Instead, its time-resolved emission resembles that of correlated systems in cases where the insulator breakdown cannot occur because  $E_{\text{th}} > E_0$ . The convergence is particularly clear as  $U/t \rightarrow \infty$ , examples of which are shown in Supplementary Fig. 5 for  $U/t_0 = 10$ . In this limit, both models show a distinctive partitioning of the HHG from different processes, as sparsely-occupied upper bands support Bloch oscillations which result in low harmonic emission, and the limited inter-band polarisation that does develop produces weak-intensity emission at large harmonics. The inter-band emission begins when the field strength is sufficient to cause excitations and continues throughout the pulse, peaking at or near the 5th cycle (where  $E(t) = E_0$ ), which is clearly distinct from the rapid onset and decay of HHG observed in systems undergoing a Mott transition (Fig. 3), where peak emission occurs soon after  $E_{\text{th}}$  is reached. These properties can be seen in Fig. 5 at effective  $U/t_0 = 7$ , whereas at  $U/t_0 = 5$  there are similar inter-band high harmonics, but Bloch oscillations are still suppressed. This confirms that when interactions are very large the sub-cycle dynamics and resulting HHG can be well-understood by considering single-particle excitations within the ground state bandstructure, in a manner comparable to some semiconductor systems [4]. Furthermore, in the large interaction regime, plateaus in the emission profile have been observed in the literature, resulting from localized doublon-hole recombination processes at different length scales on the lattice [5]. These are observed in exact diagonalization simulations in this large  $U/t_0$  limit at low intensities, and will be further investigated in future work.

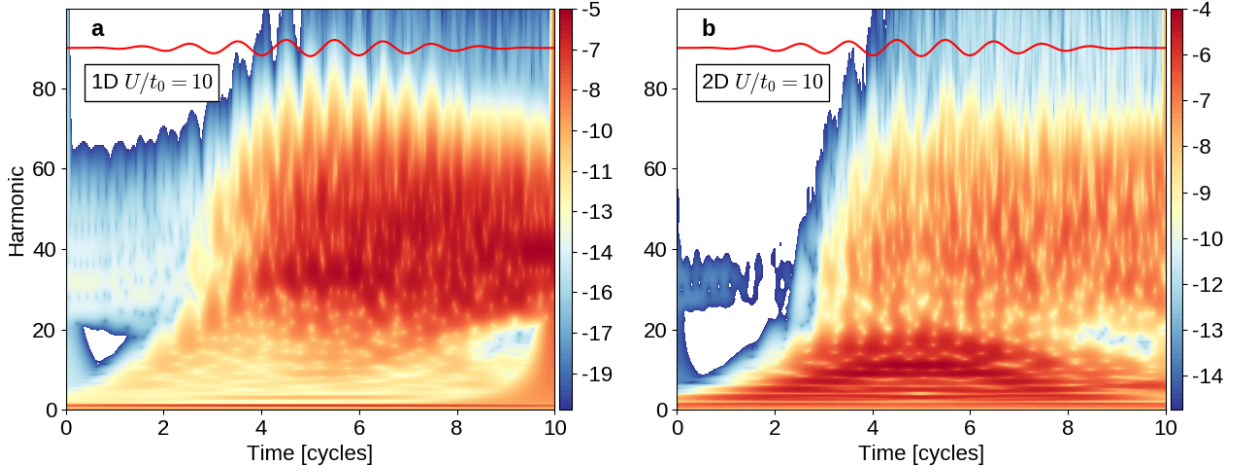

**Supplementary Fig. 5. Spectrograms in the limit of very large correlation.** HHG shows patterns of emission similar to those produced in the non-interacting model in the main text in Fig. 5. They show the time-resolved HHG at  $U/t_0 = 10$  in 1D (a) and 2D (b), calculated using ED. The red curve shows the electric field,  $E(t) = -dA(t)/dt$

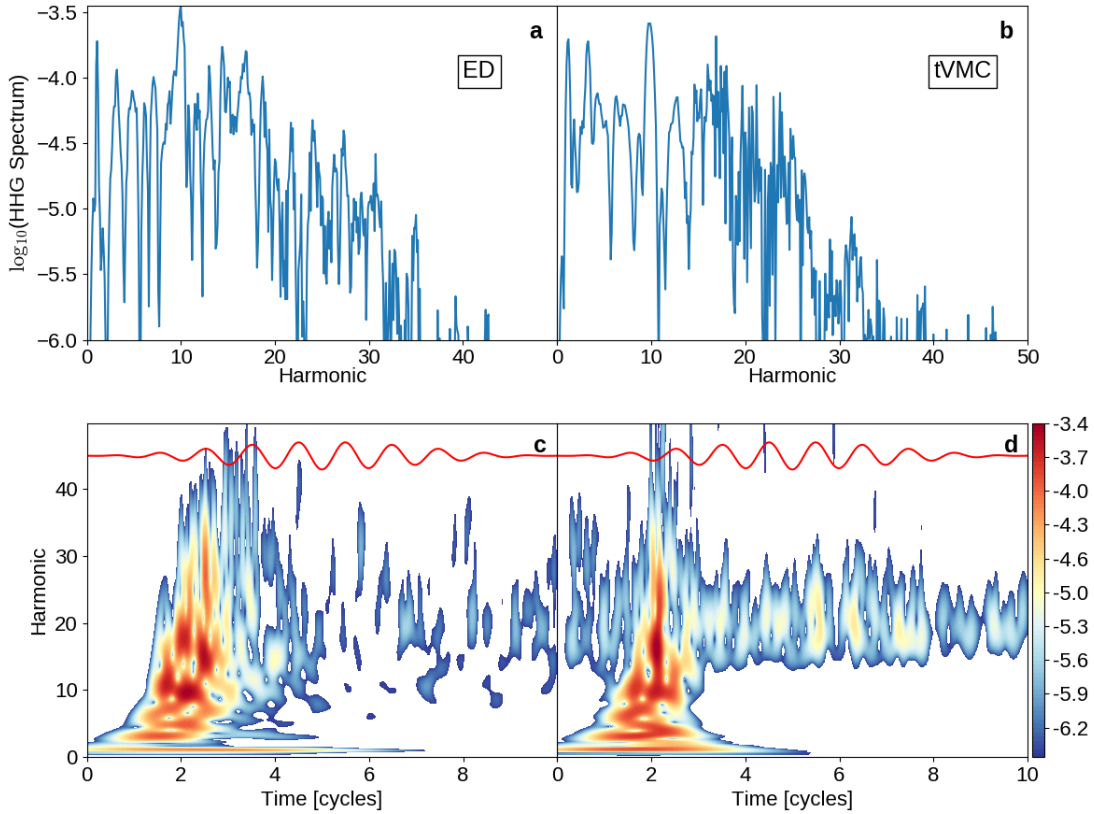

**Supplementary Fig. 6. Comparison of tVMC and ED.** HHG in the frequency and time domains in the  $4 \times 3$  system at  $U/t_0 = 5$  for ED (a,c) and tVMC (b,d).

### Benchmarking

In this section, we provide results from benchmarking of the suitability of the tVMC approach for the resulting conclusions in the main text. Firstly, tVMC simulations were compared to exact diagonalization results for the  $4 \times 3$  system, an example of which is shown in Supplementary Fig. 6 for 2D  $U/t_0 = 5$ . This shows good

agreement and the reproduction of the important qualitative features of the emission in both the time-averaged and time-resolved HHG, demonstrating the inherent suitability of the Ansatz used for the qualitative physics of HHG in Mott insulators. Secondly, we consider the convergence of the results with respect to lattice size, by

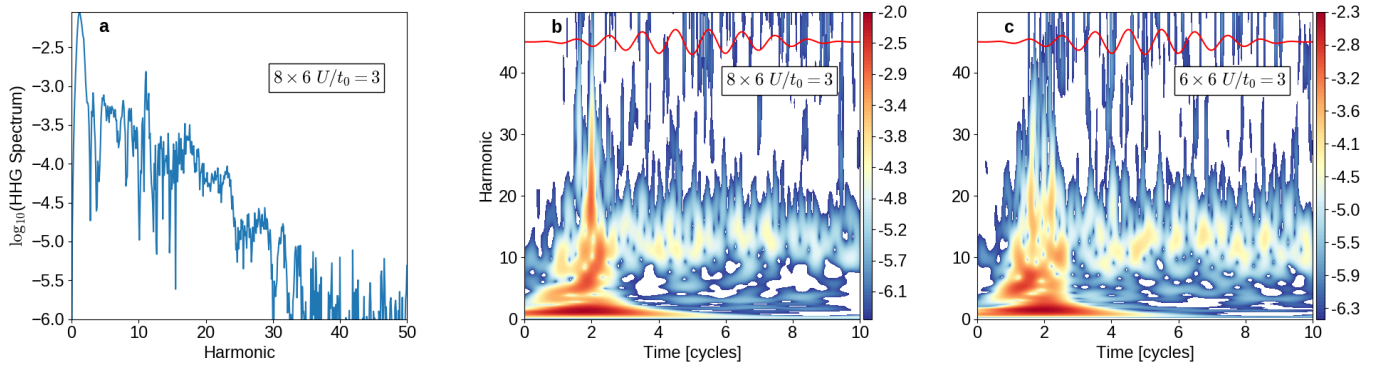

**Supplementary Fig. 7. Convergence of HHG emission profile with system size.** 2D  $U/t_0 = 3$  emission simulated in the  $8 \times 6$  lattice (a,b) and compared to the  $6 \times 6$  lattice (c) used in the rest of this work. The spectrograms exhibit the same qualitative features, while the time-averaged spectrum very closely matches the equivalent spectrum in Fig. 2 of the main text.

observing differences in the HHG emission when compared to equivalent simulations on a larger lattice. This is shown in Supplementary Fig. 7, where 2D  $U/t_0 = 3$  simulations were performed for a  $8 \times 6$  lattice, which is the largest that is reasonably attainable due to the computationally expensive form of the trial wavefunction that is required to simulate these correlated systems. We can see that the spectrograms are qualitatively unchanged compared to the  $6 \times 6$  lattice, and the time-averaged spectrum similarly reproduces the properties of its equivalent spectrum shown in Fig. 2 of the main text. Furthermore, the sensitivity of these simulations with respect to initial starting random number seed was also investigated, and found to similarly have a negligible effect on the resolution of the HHG spectra.

sion. *Phys. Rev. B*, 48:1409–1425, Jul 1993.

- [2] Masanori Kohno. Mott transition in the two-dimensional Hubbard model. *Phys. Rev. Lett.*, 108:076401, Feb 2012.
- [3] Masanori Kohno. Spectral properties near the Mott transition in the two-dimensional Hubbard model with next-nearest-neighbor hopping. *Phys. Rev. B*, 90:035111, Jul 2014.
- [4] Yuta Murakami, Shintaro Takayoshi, Akihisa Koga, and Philipp Werner. High-harmonic generation in one-dimensional Mott insulators. *Phys. Rev. B*, 103:035110, Jan 2021.
- [5] Yuta Murakami, Martin Eckstein, and Philipp Werner. High-harmonic generation in Mott insulators. *Phys. Rev. Lett.*, 121:057405, Aug 2018.

- 
- [1] C. A. Stafford and A. J. Millis. Scaling theory of the Mott-Hubbard metal-insulator transition in one dimen-
